# Supplementary material for: Piezomagnetic transport in van der Waals noncoplanar Antiferromagnets
Source: arXiv:2602.04245 ancillary file (2026-02-04)
Supplement: Supplementary file 1 [file supplement.pdf]

# Supplementary Materials: Piezomagnetic transport in van der Waals noncoplanar Antiferromagnets

Abdul Ahad[1*], Miuko Tanaka[1], Nguyen Duy Khanh[2], Riku Ishioka[2], Aki Kitaori[2], Tenta Kitamura[3], Hao Ou[3], Jiang Pu[3], Shinichiro Seki[2], Toshiya Ideue[1*]

[1]*Institute for Solid State Physics, The University of Tokyo, 5-1-5 Kashiwanoha, Kashiwa, Chiba, Japan,*

[2]*Department of Applied Physics and Quantum-Phase Electronics Center, The University of Tokyo, Tokyo, Japan,*

[3]*Department of Physics, Institute of Science Tokyo, Tokyo, Japan*

### 1. Strain estimation using bending stages.

The strain can be estimated from the radius of curvature ($R$) and the substrate thickness $t$. We assume that the substrate is bent with an arbitrary curvature, where the outer radius of curvature of the substrate is $R_2$ and the inner radius of curvature is $R_1$ ($R_2 > R_1$). The outer and inner surfaces of the substrate are subjected to opposite strains.

The strain on the outer surface can be written as

$$\varepsilon = \frac{R_2 - R_0}{R_0}, \tag{1}$$

where $R_0$ is the neutral axis, defined as

$$R_0 = \frac{R_2 + R_1}{2}.$$

Similarly, the strain on the inner surface has the same magnitude but opposite sign, given by

$$-\varepsilon = \frac{R_1 - R_0}{R_0}. \tag{2}$$

Subtracting Eq. (2) from Eq. (1), we obtain

$$2\varepsilon = \frac{R_2 - R_1}{R_0}.$$

Using the substrate thickness $t = R_2 - R_1$, the final expression for the strain is

$$\varepsilon = \frac{t}{2R_0}.$$

### 2. Thickness estimation using atomic force microscopy

We used the atomic force microscopy (AFM) (Bruker Dimension Icon) to measure the thickness of the devices. Scan Assyst mode were used. Since PEN is insulating substrate, we used the soft X-ray radiation to dissipate the charge during the AFM measurement. Thickness profiles of several micrometers were recorded to obtain the average value. Thickness of the $CoNb_3S_6$ and $CoTa_3S_6$ samples discussed in the main text are estimated as 91 nm (see Fig. S2) and 85 nm (see Fig. S3), respectively.

## 3. Piezomagnetic transport in $CoNb_3S_6$ under the in-plane strain perpendicular to the straight edge of the flake

In the main text, uniaxial strain was applied along the straight edge of the flake. According to previous research, this straight edge corresponds to a zigzag direction with a high probability [1], which we used as a reference. To check the in-plane directional dependence of strain, we performed similar measurements with the strain applied in the armchair direction. Figure S4 a show the device picture for this measurement. Figures S4 b and c represent the temperature dependence of $R_{xx}$ and magnetic field dependence of Hall resistance ($R_{yx}$) at T = 25 K under different in-plane strain magnitudes. It can be seen that strain modulation of $T_N$ and $H_c$ is similar to that observed when strain was applied in a zigzag direction is observed (Fig. S4 d and e). We note that normal Hall component ($R_{yx}^N$) obtained by fitting the high field linear region is also modulated (Fig. S4 f), indicating that strain not only change the exchange interaction but also influence the electronic structure itself.

## 4. Piezomagnetic transport in other samples of $CoTa_3S_6$ under the in-plane strain parallel and perpendicular to the straight edge of the flake

We measured piezomagnetic transport also in other samples of $CoTa_3S_6$ under different uniaxial strain directions (Figs. S5 a and d). For the sample shown in Fig. S5 a, we applied uniaxial strain perpendicular to the straight edge of the sample. Similar to the samples discussed in the main text, in which strain is applied parallel to the straight edge, coercive field is systematically modulated, showing the linear dependence on the strain (Figs. S5 b and c). This result suggests that, similar to the previously mentioned $CoTa_3S_6$, strain in the zigzag direction and armchair direction produces similar responses. For the sample shown in Fig. S5 d, uniaxial strain parallel to the straight edge was applied, similar to the samples discussed in this paper. As shown in Fig. S5 e, strain-switchable trend in temperature variation of resistance, which may come from the nematic domain control, has been observed also in this sample. At the intermediate temperature between $T_{N1}$ and $T_{N2}$ (T = 30 K) we evaluated the pressure variation of the normal Hall coefficient. It also shows systematic modulation by strain, indicating that strain not only changes the exchange interaction but also influences the electronic structure itself.

### 5. Spontaneous Hall resistivity ($\rho_{yx}^{SHE}$), and longitudinal resistance ($\rho_{xx}$) of $CoNb_3S_6$

Figure S6 a, comprises the temperature dependence of zero field Hall resistivity under different uniaxial in-plane strain. It is recorded by field cooling process; after cooling the sample under the magnetic field (B = - 9 T), $\rho_{yx}^{SHE}$ was measured under zero field while warming. On the one hand, the magnitude of $\rho_{yx}^{SHE}$ saturates below around 10 K, showing value almost independent of strain value. On the other hand, the magnitude of $\rho_{xx}$ is strain sensitive throughout the temperature range (see Fig. S6 b), which is the cause of the sysytematic strain modulation of $\sigma_{xy}^{SHE}$ discussed in the main text.

### 6. Piezomagnetic tensor for $CoM_3S_6$ (M = Nb, Ta)

From neutron diffraction studies [2, 3] on $CoM_3S_6$ (M = Nb, Ta), the deduced magnetic point group in the all-in–all-out (AIAO) phase is $32'$. The piezomagnetic effect can be described as $M = \Lambda\epsilon$, where the magnetization $M$ is induced by the strain $\epsilon$. The piezomagnetic tensor $\Lambda$ is an axial tensor. In matrix form, it can be expressed as [4]

$$\begin{pmatrix} M_x \\ M_y \\ M_z \end{pmatrix} = \begin{pmatrix} 0 & 0 & 0 & 0 & \Lambda_{15} & \Lambda_{16} \\ \Lambda_{16} & -\Lambda_{16} & 0 & \Lambda_{15} & 0 & 0 \\ \Lambda_{31} & \Lambda_{31} & \Lambda_{33} & 0 & 0 & 0 \end{pmatrix} \begin{pmatrix} \varepsilon_{xx} \\ \varepsilon_{yy} \\ \varepsilon_{zz} \\ \varepsilon_{yz} \\ \varepsilon_{xz} \\ \varepsilon_{xy} \end{pmatrix}$$

Here, Voigt notation is used, such that $\Lambda_{\alpha\beta} \to \Lambda_{ijk}$, with $\alpha \to i$ and $\beta \to jk$. Note that the above form leads to $\Lambda_{zxx} = \Lambda_{zyy} (= \Lambda_{31})$, which is consistent with the results that piezomagnetic transport seems to independent of the in-plane direction of the uniaxial strain.

### 7. Piezomagnetic effect in non-coplanar spin systems

In collinear magnetic structures, it has been realized that the canting of magnetic moments due to uneven exchange interactions under strain is the main source of piezomagnetism. Considering a similar situation in the present case, piezomagnetism can also arise in non-coplanar spin systems. In the schematic shown in Fig. S7, four spin vectors in the all-

in–all-out configuration are labeled as $M_n$ ($n = 1$ to 4). The vector $M_1$ is aligned along the $z$ axis, while the other spins make an angle $\theta$ with $M_1$. For a regular tetrahedron, $\theta \approx 109.5°$. For the all-in–all-out spin configuration, the local magnetic moments of magnitude $m$ are defined as follows [2]:

$$M_1 = m e_z, \tag{1}$$

$$M_2 = m\left(e_y \sin\theta + e_z \cos\theta\right), \tag{2}$$

$$M_3 = m\left(e_x \frac{\sqrt{3}}{2}\sin\theta - e_y \frac{1}{2}\sin\theta + e_z\cos\theta\right), \tag{3}$$

$$M_4 = m\left(-e_x \frac{\sqrt{3}}{2}\sin\theta - e_y \frac{1}{2}\sin\theta + e_z\cos\theta\right), \tag{4}$$

where $e_x$, $e_y$, and $e_z$ are the unit vectors along the $x$, $y$, and $z$ directions, respectively.

The exchange energy can be written using the Heisenberg Hamiltonian [5] as

$$E = -\sum_{i,j}^{i,j=4} J_{ij}\, M_i \cdot M_j,$$

where $J_{ij}$ denotes the nearest-neighbor exchange interaction (e.g., $J_{12}$).

Explicitly, the total exchange energy is given by

$$\begin{aligned} E = &- J_{14} M_1 \cdot M_4 - J_{24} M_2 \cdot M_4 - J_{34} M_3 \cdot M_4 \\ &- J_{12} M_1 \cdot M_2 - J_{23} M_2 \cdot M_3 - J_{13} M_1 \cdot M_3. \end{aligned} \tag{5}$$

Substituting Eqs. (1)–(4) into Eq. (5), the exchange energy becomes

$$\begin{aligned} E = &- J_{14}\cos\theta - J_{13}\cos\theta - J_{12}\cos\theta \\ &- J_{23}\left(-\frac{1}{2}\sin^2\theta + \cos^2\theta\right) \\ &- J_{24}\left(-\frac{1}{2}\sin^2\theta + \cos^2\theta\right) \\ &- J_{34}\left(-\frac{1}{2}\sin^2\theta + \cos^2\theta\right). \end{aligned} \tag{6}$$

By assuming $J_{14} = J_{13} = J_{12} = J_c$ and $J_{23} = J_{24} = J_{34} = J_{ab}$, Eq. (6) leads to the following relation.

$$E = -3J_c\cos\theta - 3J_{ab}\left(-\frac{1}{2}\sin^2\theta + \cos^2\theta\right). \quad (7)$$

Under the application of strain, $J_c$ and $J_{ab}$ will be modulated, thus the angle $\theta$ will also change accordingly to minimize the exchange energy.

By minimizing the exchange energy, *i.e.*, $\partial E/\partial\theta = 0$, we will get the following relation between exchange $J_c$ and $J_{ab}$.

$$J_c + 3J_{ab}\cos\theta = 0. \quad (8)$$

We can define the magnitude $m_{net}$ in the $z$ direction as,

$$m_{\rm net} = m + 3m\cos\theta.$$

Using Eq. (8),

$$m_{\rm net} = m\left(1 - \frac{J_c}{J_{ab}}\right).$$

Assuming the change of exchange interaction under compressive strain as $J_c = J_0 - \Delta J$ and $J_{ab} = J_0 + \Delta J$, we get the final relation of strain induced $m_{net}$ as

$$m_{\rm net} \simeq m\left(\frac{2\Delta J}{J_0}\right),$$

Here in the denominator, we use the approximation $J_0 \pm \Delta J \approx J_0$, as the $\Delta J$ is small.

Similarly, under the tensile strain, assuming the change of the exchange interactions as $J_c = J_0 + \Delta J$ and $J_{ab} = J_0 - \Delta J$, leading to the strain induced $m_{net}$ as:

$$m_{\rm net} \simeq -m\left(\frac{2\Delta J}{J_0}\right).$$

This relation implies that the imbalance between exchange interaction is important for piezomagnetism.

### 8. Temperature variation of coercive field and its strain dependence in $CoNb_3S_6$

In the case of $CoNb_3S_6$, coercive field dramatically increases upon cooling the system6. For unstrained case ($\epsilon$ = 0 %), because of the large $H_c$, we cannot observe the switching behavior in Hall resistance even at $T$ = 23 K ($H_c$ > 8 T at $T$ = 23 K). However, the

application of compressive strain reduces the $H_c$ significantly and made it possible to observe the domain switching at T = 22 K (Fig. S8 a). In Fig. S8 b, we compare the temperature variation of coercive field under $\epsilon$ = 0 % and $\epsilon$ = -1 %, which clearly shows the large modulation of $H_c$ under strain.

## 9. Magnetoresistance of $CoNb_3S_6$ and its strain dependence

As the main observation of this work is piezomagnetic control over the Berry curvature related transport, we did not discuss the longitudinal transport and its strain dependence in the main text. In Fig. S9 we plot the magnetoresistance $\frac{(R_{xx}(H)-R_{xx}(0))}{(R_{xx}(0))}$ , recorded at 25 K under several strain values (-1.5 % to +1.5 %). It is noted that very small magnetoresistance is observed in our samples without strain, which is consistent with previous study of bulk single crystal [6]. Moreover, it does not show significant strain dependence.

## 10. Temperature variation of coercive field and its strain dependence in $CoTa_3S_6$

In the case of $CoTa_3S_6$, unlike the $CoNb_3S_6$, swithcing behavior in Hall resistance is measurable even at 5 K. Figs. S10 a and b show the strain evolution of $H_c$ at T = 5 K and 10 K, respectively. It should be noted that strain dependence of $H_c$ is opposite from $CoNb_3S_6$; *i.e.*, tensile strain casue the decrease of $H_c$ in the case of $CoTa_3S_6$. Figure S10 c shows the temperature variation of coercive field for $\epsilon$ = -1 %, 0 % and 1 %, alongwith the single crystal data [7].

## 11. Potential piezomagnetic switching of antiferromagnetic domains for straintronics memory devices

In this work, we demonstrate the strain tunable coercive field. This means that antiferromagnetic domains can be controlled by strain at the fixed magnetic field. For example, starting from state 1 (red point in Fig. S11) and changing the strain value (from compressive to tensile strain), we can switch the antiferromagnetic domains, obtaining state 0 (yellow point in Fig. S11) This type of functionality of antiferromagnetic domain control by strain

can be applicable to the future straintronic memory devices.

---


[1] Y. Guo *et al.*, ACS Nano **10**, 8980–8988 (2016).

[2] H. Takagi *et al.*, Nat. Phys. **19**, 961–968 (2023).

[3] P. Park *et al.*, Nat. Commun. **14**, (2023).

[4] S. V. Gallego, J. Etxebarria, L. Elcoro, E. S. Tasci, and J. M. Perez-Mato, Acta Crystallogr. A **75**, 438–447 (2019).

[5] J. Zemen, Z. Gercsi, and K. G. Sandeman, Phys. Rev. B **96**, (2017).

[6] N. J. Ghimire *et al.*, Nat. Commun. **9**, (2018).

[7] P. Park *et al.*, npj Quantum Mater. **7**, (2022).

## SUPPLEMENTARY FIGURES

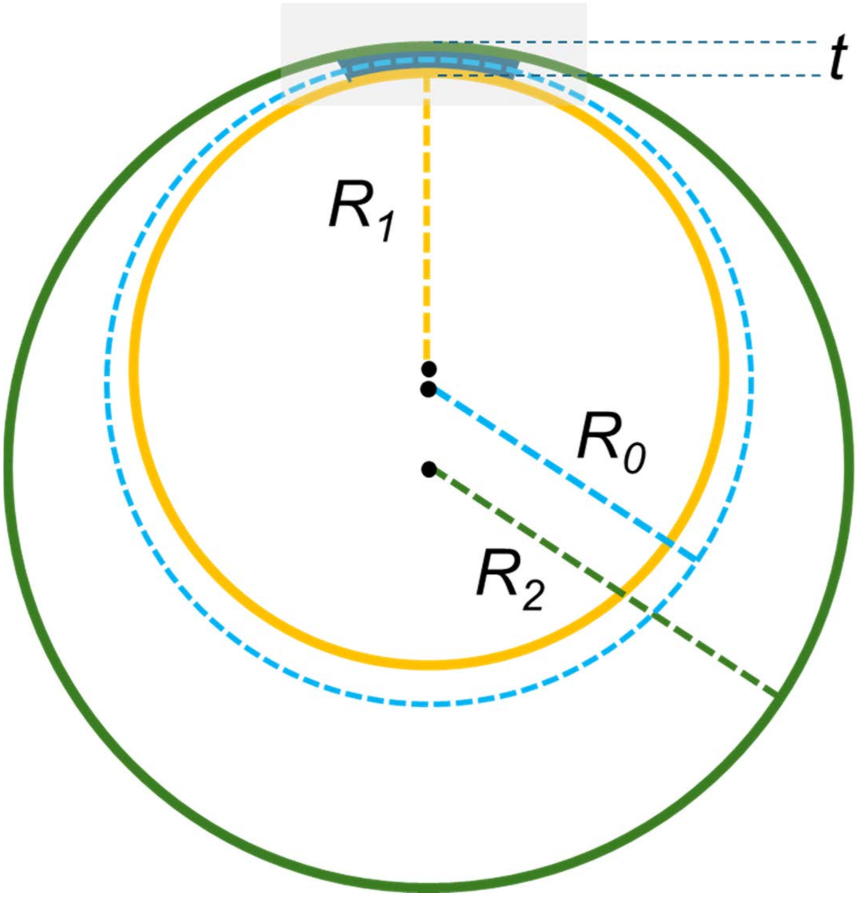


Supplementary Fig. 1. **Strain estimation using bending stage.**

Schematics of the outer and inner surface of a bent substrate (dark blue in shaded region). The outer radius is $R_2$ (green circle) while inner one (orange circle) is $R_1$ due to strain. The neutral axis radius (dashed blue circle) is the arithmetic mean of $R_1$ and $R_2$. The thickness of the substrate is defined as $R_2 - R_1$.

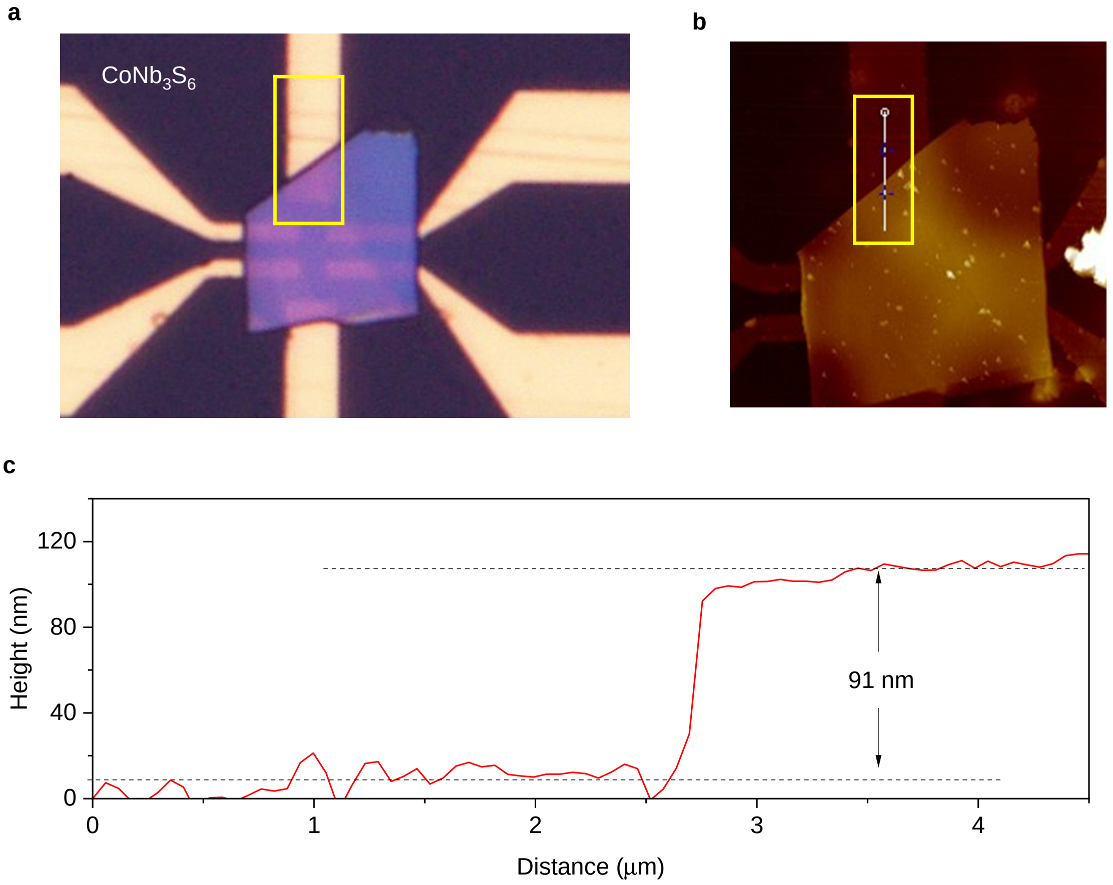


Supplementary Fig. 2. **AFM measurement of $CoNb_3S_6$ device.**

**a** The optical microscope image of the $CoNb_3S_6$ device. **b** AFM topography image of the device. **c** Height profile along the dashed line in the yellow rectangle in b.

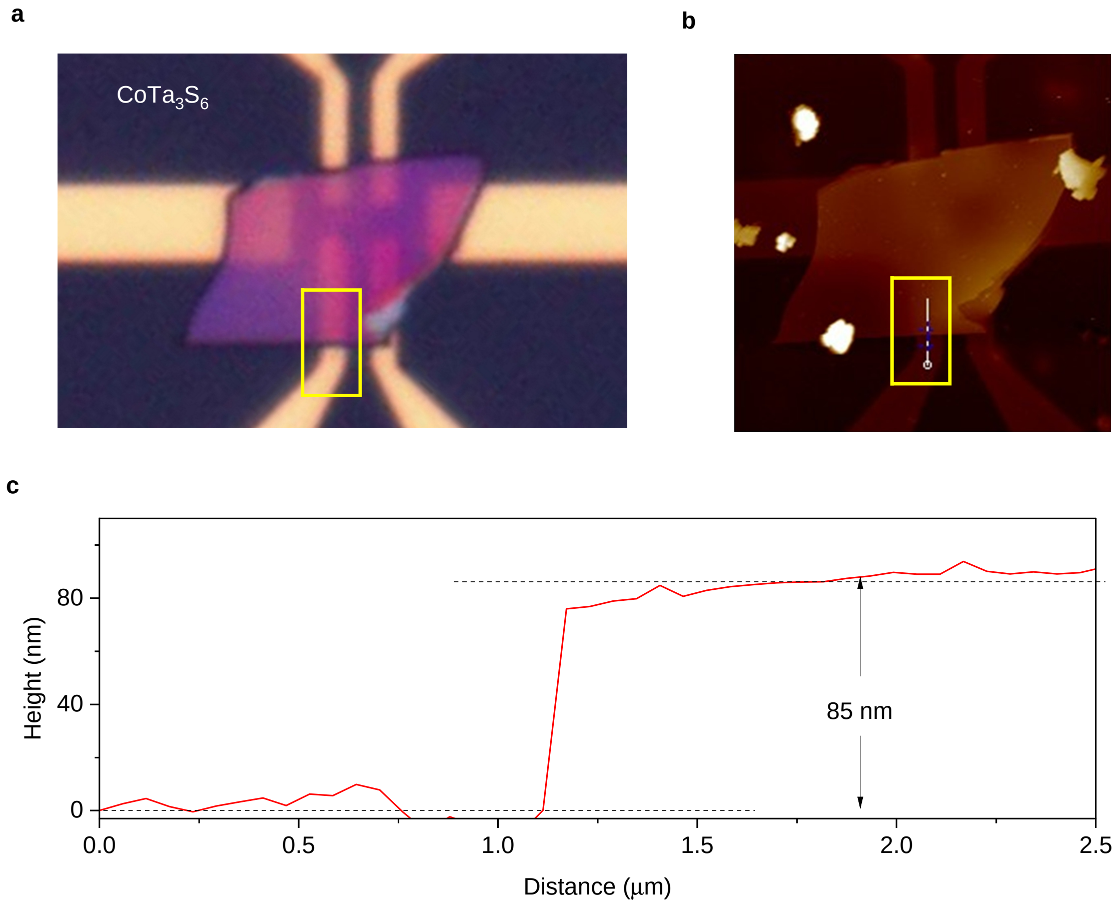


Supplementary Fig. 3. **AFM measurement of $CoTa_3S_6$ device.**

**a** The optical microscope image of the $CoTa_3S_6$ device. **b** AFM topography image of the device. **c** Height profile along the dashed line in the yellow rectangle in b.

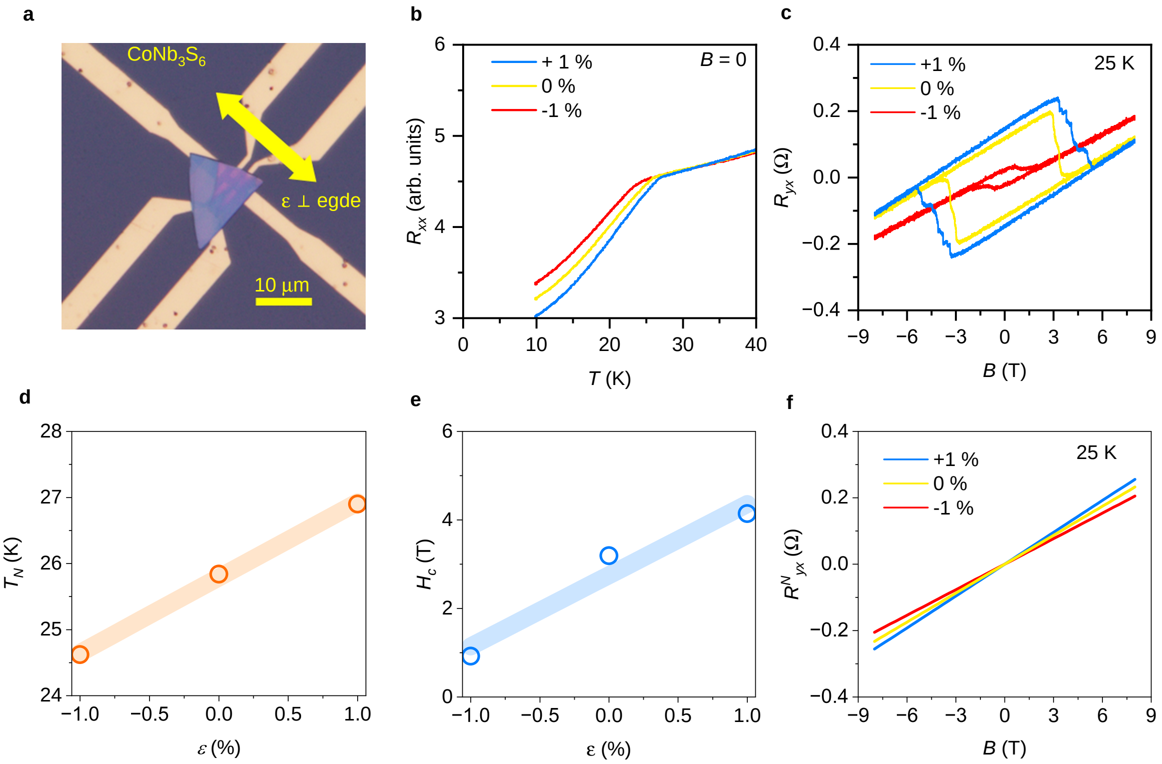


Supplementary Fig. 4. **Piezomagnetic transport in $CoNb_3S_6$ under the in-plane strain perpendicular to the straight edge of the flake.**

**a** The optical microscope image of the $CoNb_3S_6$ with the in-plane strain direction perpendicular to the straight edge of the flake. **b** Temperature dependence of resistance ($B = 0$), **c** Magnetic field dependence of Hall resistance at T = 25 K under strain. **d**, **e** Strain variation of the Neel temperature $T_N$ (d) and coercive field $H_c$ (e). **f** Normal Hall component deduced from the fitting in the high field linear region at T = 25 K under several strain values.

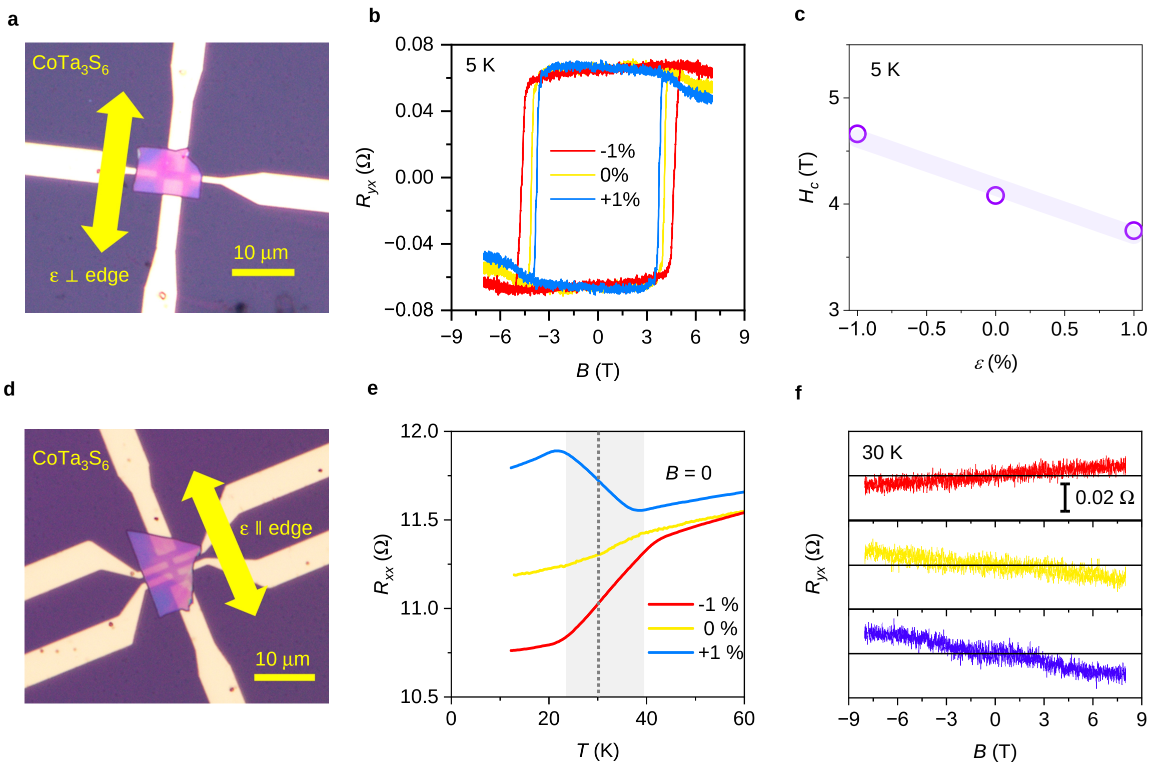


Supplementary Fig. 5. **Piezomagnetic transport in other samples of $CoTa_3S_6$.**

**a** The optical microscope image of the $CoTa_3S_6$ with the in-plane strain direction perpendicular to the straight edge of the flake. **b** Magnetic field dependence of Hall resistance (at 5 K) under strain. **c** Strain dependence of the coercive field obtained from b. **d** The optical microscope image of the $CoTa_3S_6$ with the in-plane strain direction parallel to the straight edge of the flake. **e** Temperature dependence of the $R_{xx}$ under strain. Grey shaded area indicates the region between $T_{N1}$ and $T_{N2}$. **f** Normal Hall component obtained from the data at T = 30 K (dashed black line in e).

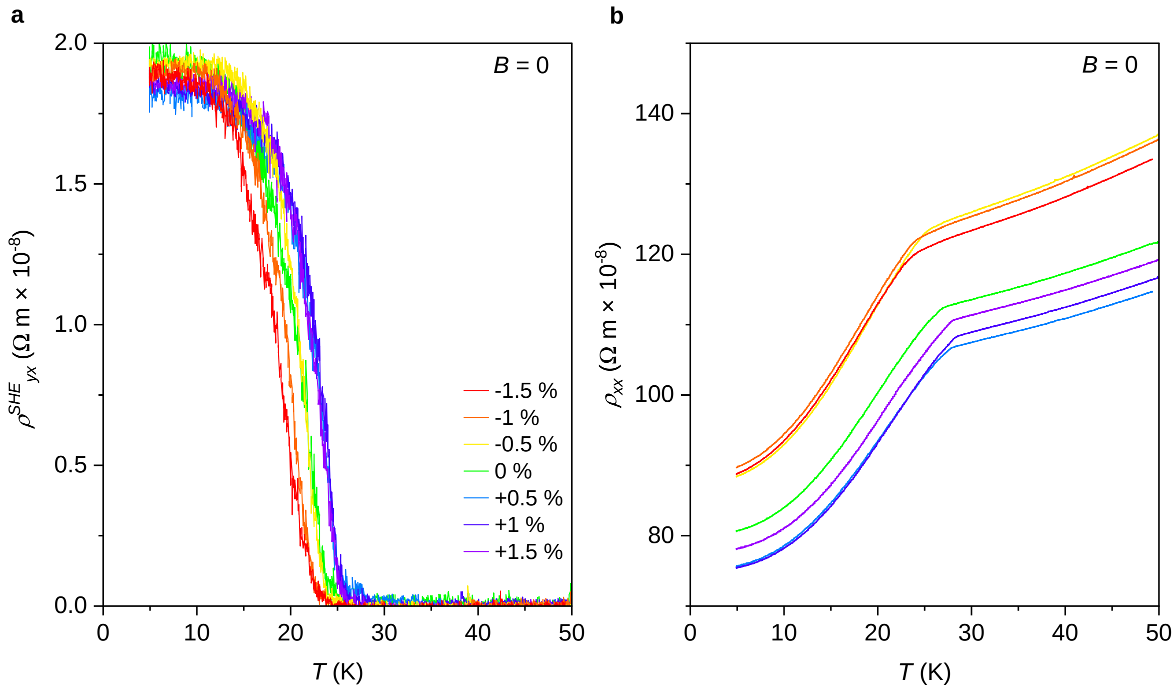


Supplementary Fig. 6. **Temperature dependent $\rho_{yx}^{SHE}$ and $\rho_{xx}$ of $CoNb_3S_6$.**

**a** Temperature dependence of zero field spontaneous Hall resistivity under different in-plane strain. Below 10 K, $\rho_{yx}^{SHE}$ saturates, showing value almost independent of applied strain however the change in $T_N$ is visible. **b** Temperature dependence of resistivity. It shows systematic modulation by strain.

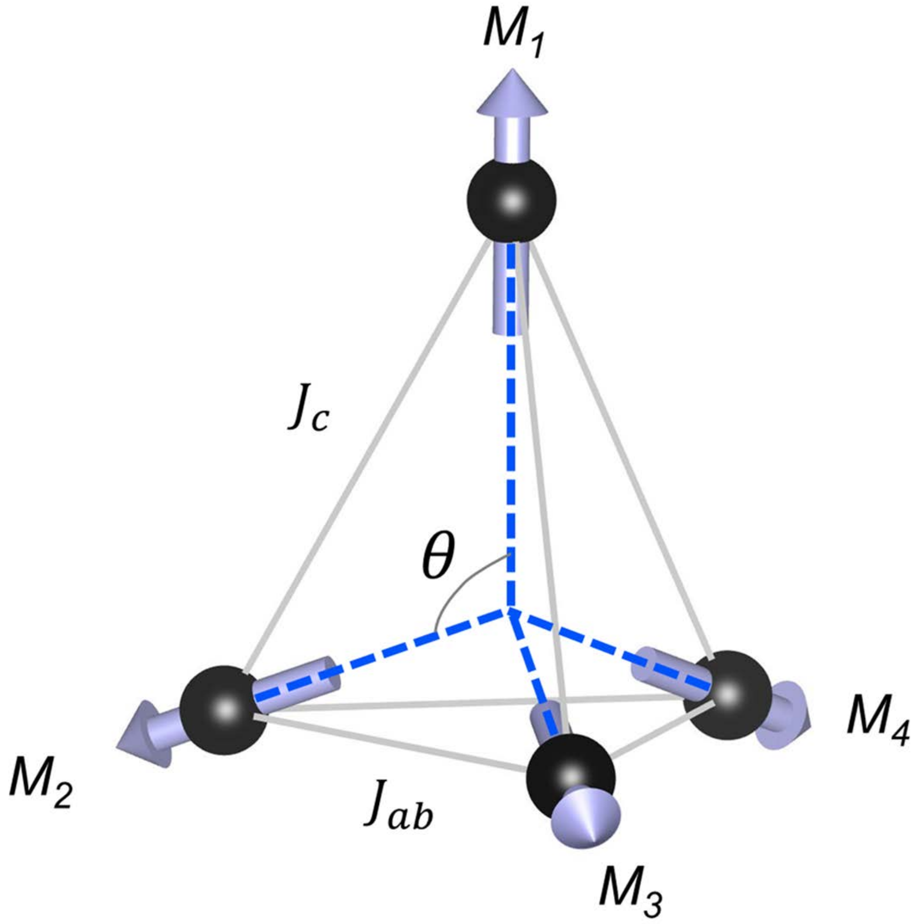


Supplementary Fig. 7. **Piezomagnetism in non-coplaner spin systems.**

Schematic of four spins unit tetrahedra in all-in-all-out spin configuration. The $\theta$ is the angle between the local magnetic moment vector $M_1$ and $M_n$ (n =2,3 and 4). The out of plane and in-plane exchange interactions are denoted by $J_c$ and $J_{ab}$, respectively.

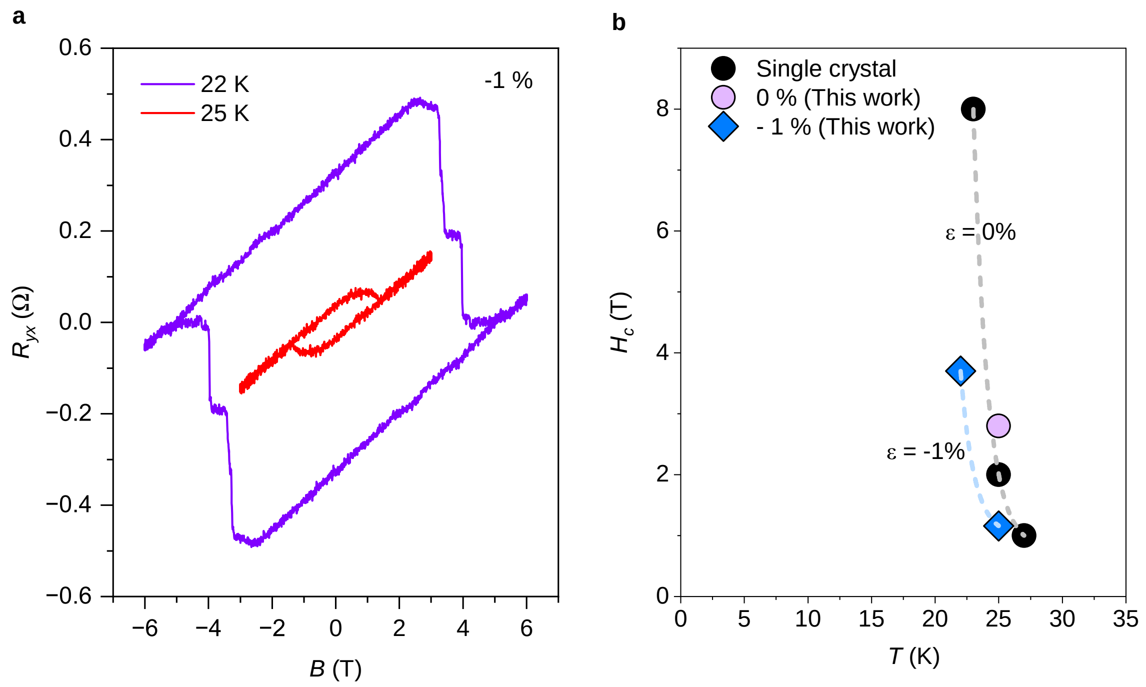


Supplementary Fig. 8. **Temperature variation of coercive field in $CoNb_3S_6$.**

**a** Hall resistance ($R_{yx}$) in strained $CoNb_3S_6$ ($\epsilon$ = -1 %) at T = 22 K and 25 K while sweeping magnetic field. Clear switching behavior, which cannot be observed in unstrained samples due to the large $H_c$, can be detected. **b** Temperature variation of coercive field and its strain dependence. The single crystal data is adopted from the previous report [Ref. 6]. Dashed lines are the guide to the eye.

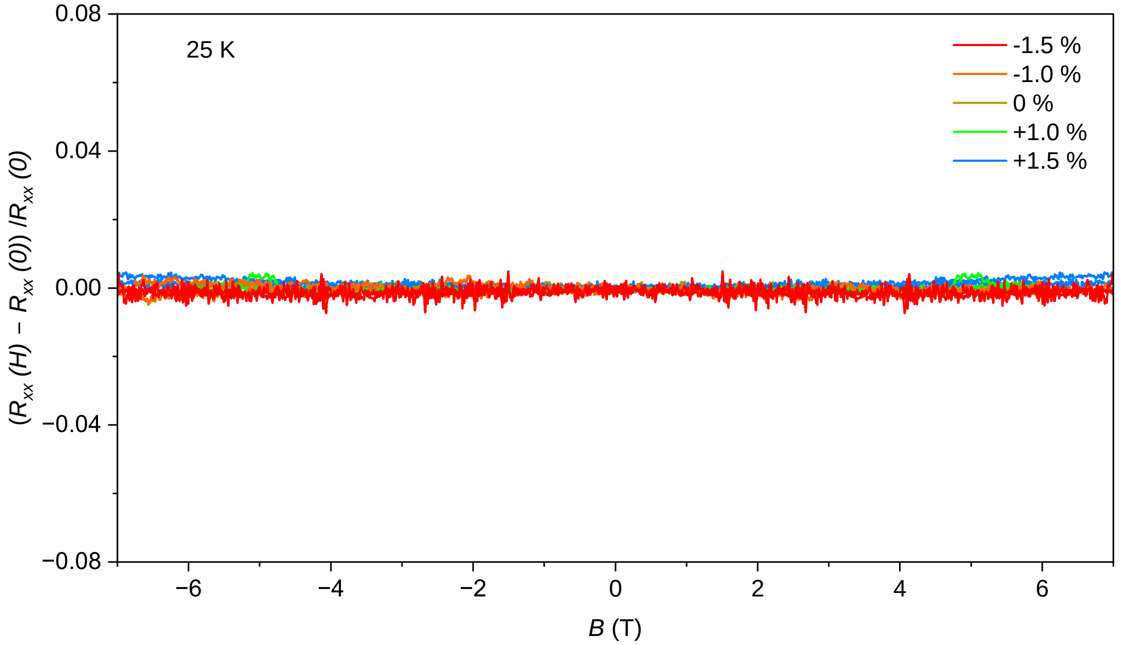


Supplementary Fig. 9. **Magnetoresistance of $CoNb_3S_6$ and its strain dependence.** Magnetoresistance $((R_{xx}(H) - R_{xx}(0))/(R_{xx}(0)))$ recorded at various strain magnitudes ranging from -1.5 % to +1.5 % while sweeping the field at $T = 25$ K.

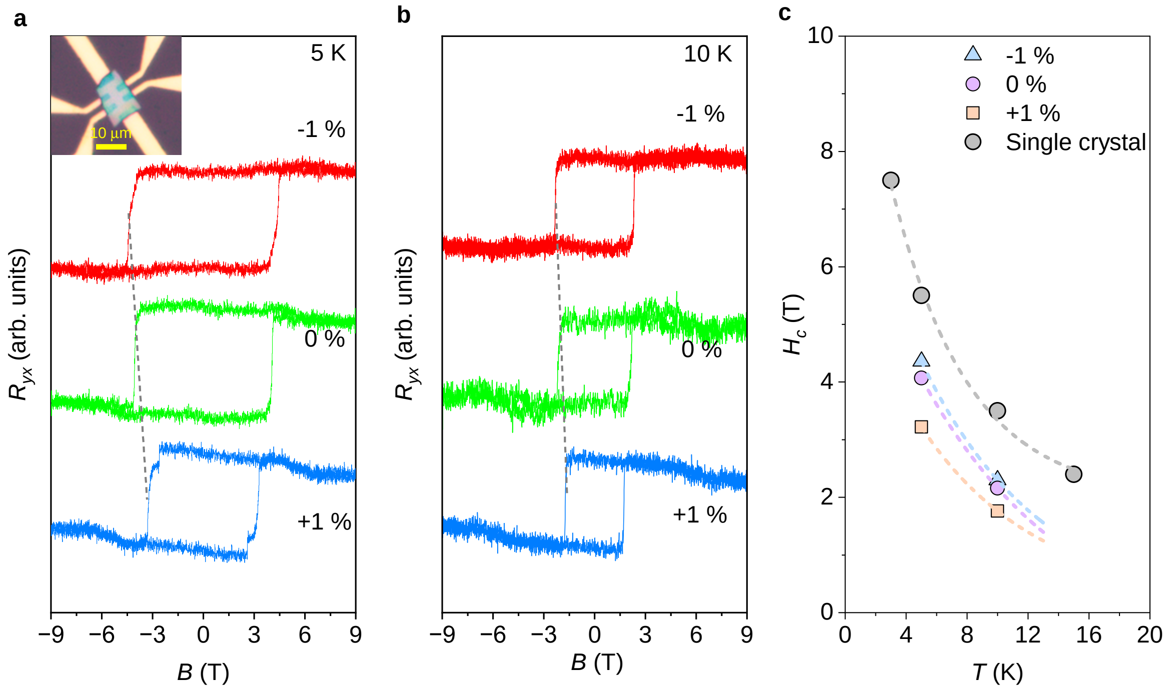


Supplementary Fig. 10. **Temperature variation of coercive field in $CoTa_3S_6$.**
**a-b** Hall resistance ($R_{yx}$) measured in $CoTa_3S_6$ at T = 5 K (a) and 10 K (b) under several strain values. **c** Temperature variation of coercive field and its strain dependence. The single crystal data is adopted from the previous report [Ref. 7]. Dashed lines are the guide to the eye.

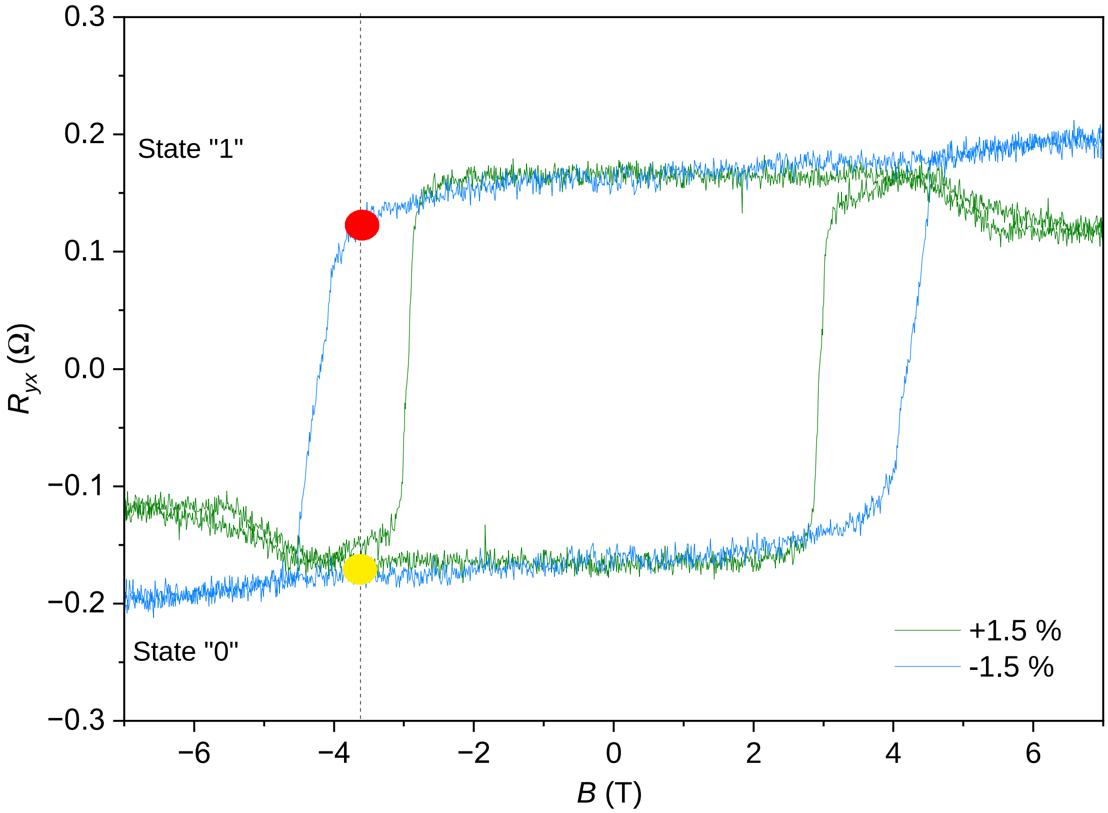


Supplementary Fig. 11. **Possible antiferromagnetic domain switching by strain in $\mathbf{CoTa_3S_6}$.**

By using the strain-tunable coercive field, it may be possible to control the antiferromagnetic domains by strain at the fixed magnetic field.
